# Supplementary material for: DiffStyler: Controllable Dual Diffusion for Text-Driven Image Stylization
Source: arXiv:2211.10682 source file (2023-12-18)
Supplement: Supplementary file 1 [file appendix.tex]

% \appendix

% \section{More Implementation Details}
% A 602M parameter CLIP conditioned model trained on Conceptual 12M for 3.1M steps and then fine-tuned for classifier-free guidance for 250K additional steps. 

\section{Additional Ablation Study}
\subsection{Effect of the CLIP Guidance Scale}
CLIP guidance scale $\lambda_d$ determines how consistently the results match the text prompts. We compared the generated results by taking different $\lambda_d$ values to verify the impact of text guidance. As shown in Fig.~\ref{fig:clip_guidance}, the generated results are more consistent with the input content image when using a smaller $\lambda_d$. As $\lambda_d$ is gradually increased, the generated results are brought closer to the semantic content of the prompt and the user's requirements. However, when the value of $\lambda_d$ is too large, the discrepancy between the stylized result and the content of the input image increases, which will cause the stylization to fail. Therefore, with an appropriate CLIP guidance scale value, the result can be made to match the text prompt content while keeping the content of the input image.

% \subsection{Learnable Noise}
\input{Figures_sup/clip_guidance}
\input{Figures_sup/steps}
\input{Figures_sup/failure_cases}
\input{Figures_sup/sup_comparison1}
\input{Figures_sup/sup_comparison2}

\subsection{Effect of the Inference Steps}
To ensure the quality of the results and to keep the consistency of the parameters, the number of free diffusion steps $T_1$ used in the experiments in this work is 150 and the number of inference process steps $T$ is $50$. The number of steps determines the quality of the generation and the length of the generation time. We found experimentally (see Fig.~\ref{fig:steps}) that the number of inference steps $T$ is set to $50$, and we can obtain good results. When the number of inference steps is larger than $50$, the result changes are no longer significant and converge to the upper mass limit.

\section{More Results}
\subsection{More results of \shortname}
The additional stylization results of \shortname are presented in Figs.~\ref{fig:diversity1}, \ref{fig:diversity2}, \ref{fig:diversity3}, \ref{fig:moreresults1}, \ref{fig:moreresults2} and \ref{fig:moreresults3}. These results demonstrate the performance of our model in terms of diversity and quality.

\subsection{Generated-based Baseline}
We compare the proposed \shortname with additional baseline ``generation-stylization'', applying the image generated by the text-to-image generation model as the style image and then performing style transfer. 
We use VQGAN-CLIP~\cite{vqganclip}, Midjourney Diffusion~\cite{midjourney} and Stable Diffusion~\cite{latentdiffusion} generated images as style images. In addition, we choose the arbitrary style transfer model AdaAttN~\cite{liu2021adaattn} as the style transfer method.

In Figs.~\ref{fig:sup-baseline1} and \ref{fig:sup-baseline2}, we can observe that the stylized methods do not adequately represent the detailed differences between the different generated results. In particular, there are clear traces of contouring between the foreground and the background, which leads to a gap between the stylized result and the real artwork.

\subsection{Failure Cases}
Although we present high-quality results for a single text condition, our approach is not without limitations. In particular, the input may not be fully preserved in the results. In this section, we show several failure cases of our model. As shown in Fig.~\ref{fig:failurecase}, the cat's fur disappears to some extent in the first row; the distinction between ``river'', ``land'' and ``mountain'' is no longer obvious in the second row; the windows of the house disappear in the third row. We found that the generated results are more focused on what is mentioned in the text, and what is not covered is potentially disappearing.

\section{Social Impact}
We explored the ability of machines to create high-quality stylized works with textual guidance and eventually achieved surprising results. In this work, we primarily use two pre-trained models, CLIP and diffusion models. CLIP~\cite{clip}, trained on 400 million image-text pairs from the Internet, introduces bias despite the large number. The diffusion model we used, trained on the CC12M~\cite{changpinyo2021cc12m} dataset and the WikiArt~\cite{WikiArt} dataset, produces biased results during iterations.
\shortname is capable of stylized editing of arbitrary content images using arbitrary textual cues. When users input arbitrary content images and text prompts, there may be negative social implications. We recommend that users use \shortname in the correct way.

\input{Figures_sup/diversity1}
\input{Figures_sup/diversity2}
\input{Figures_sup/diversity3}
\input{Figures_sup/moreresults1}
\input{Figures_sup/moreresults2}
\input{Figures_sup/moreresults3}
